# Supplementary material for: X$^3$KD: Knowledge Distillation Across Modalities, Tasks and Stages for Multi-Camera 3D Object Detection
Source: arXiv:2303.02203 source file (2023-03-03)
Supplement: Supplementary file 1 [file supp_qualitative.tex]

\section{Qualitative Analysis}

\begin{figure*}
    \captionsetup{font=small, belowskip=-12pt}
    \centering
    \includegraphics[width=0.96\linewidth]{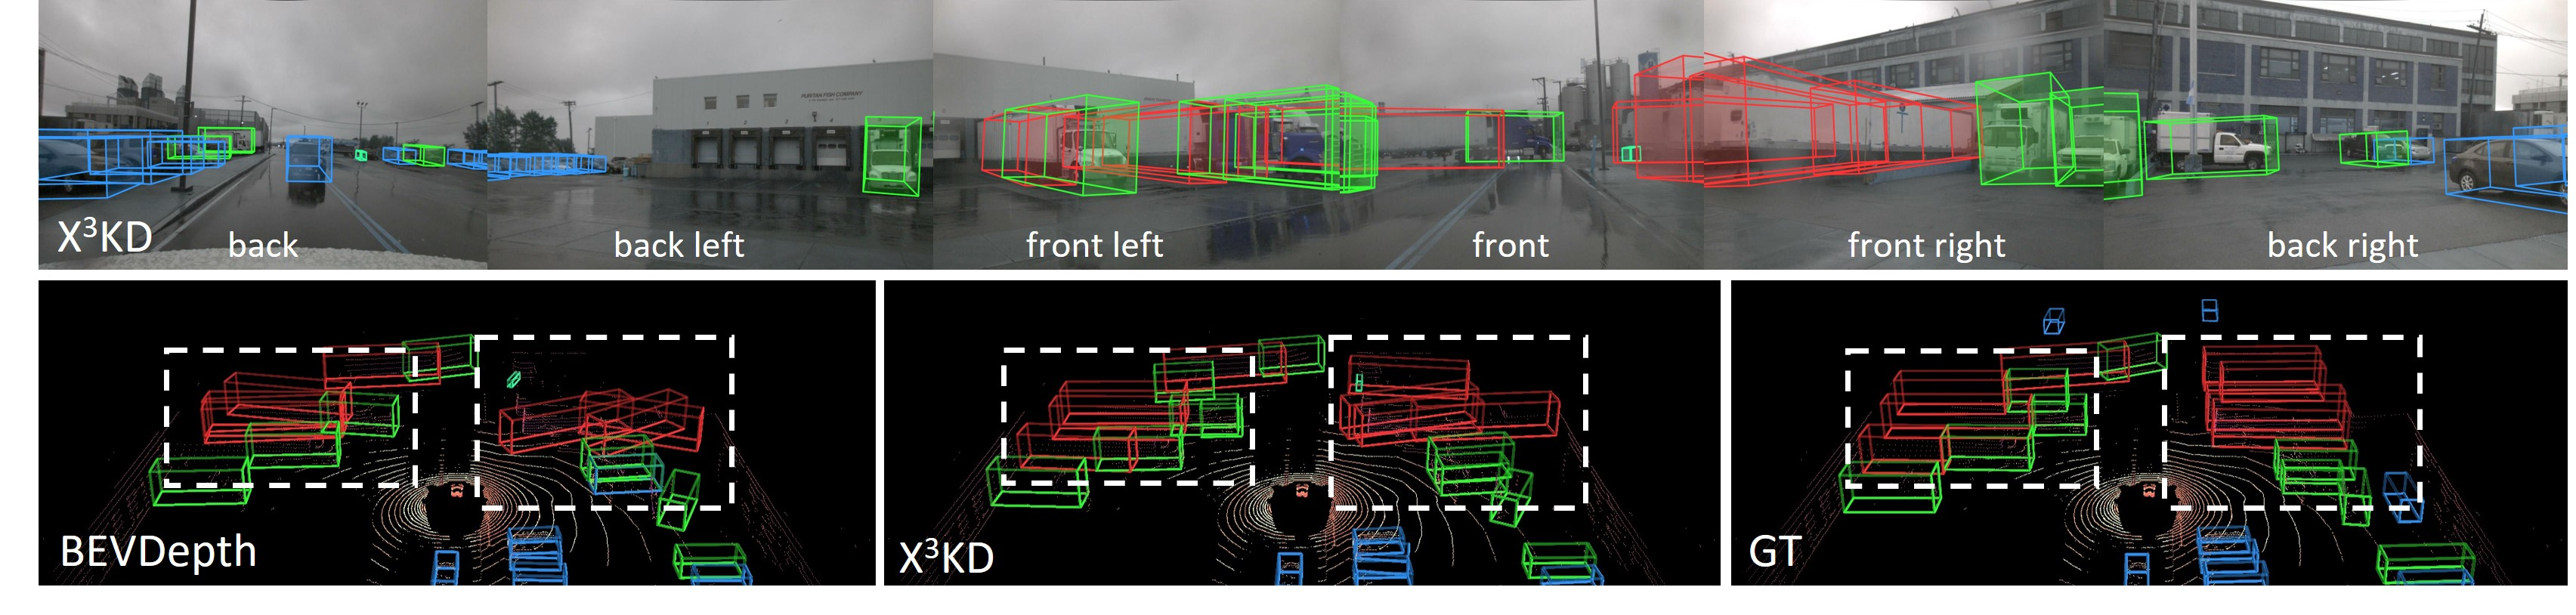}
    \includegraphics[width=0.96\linewidth]{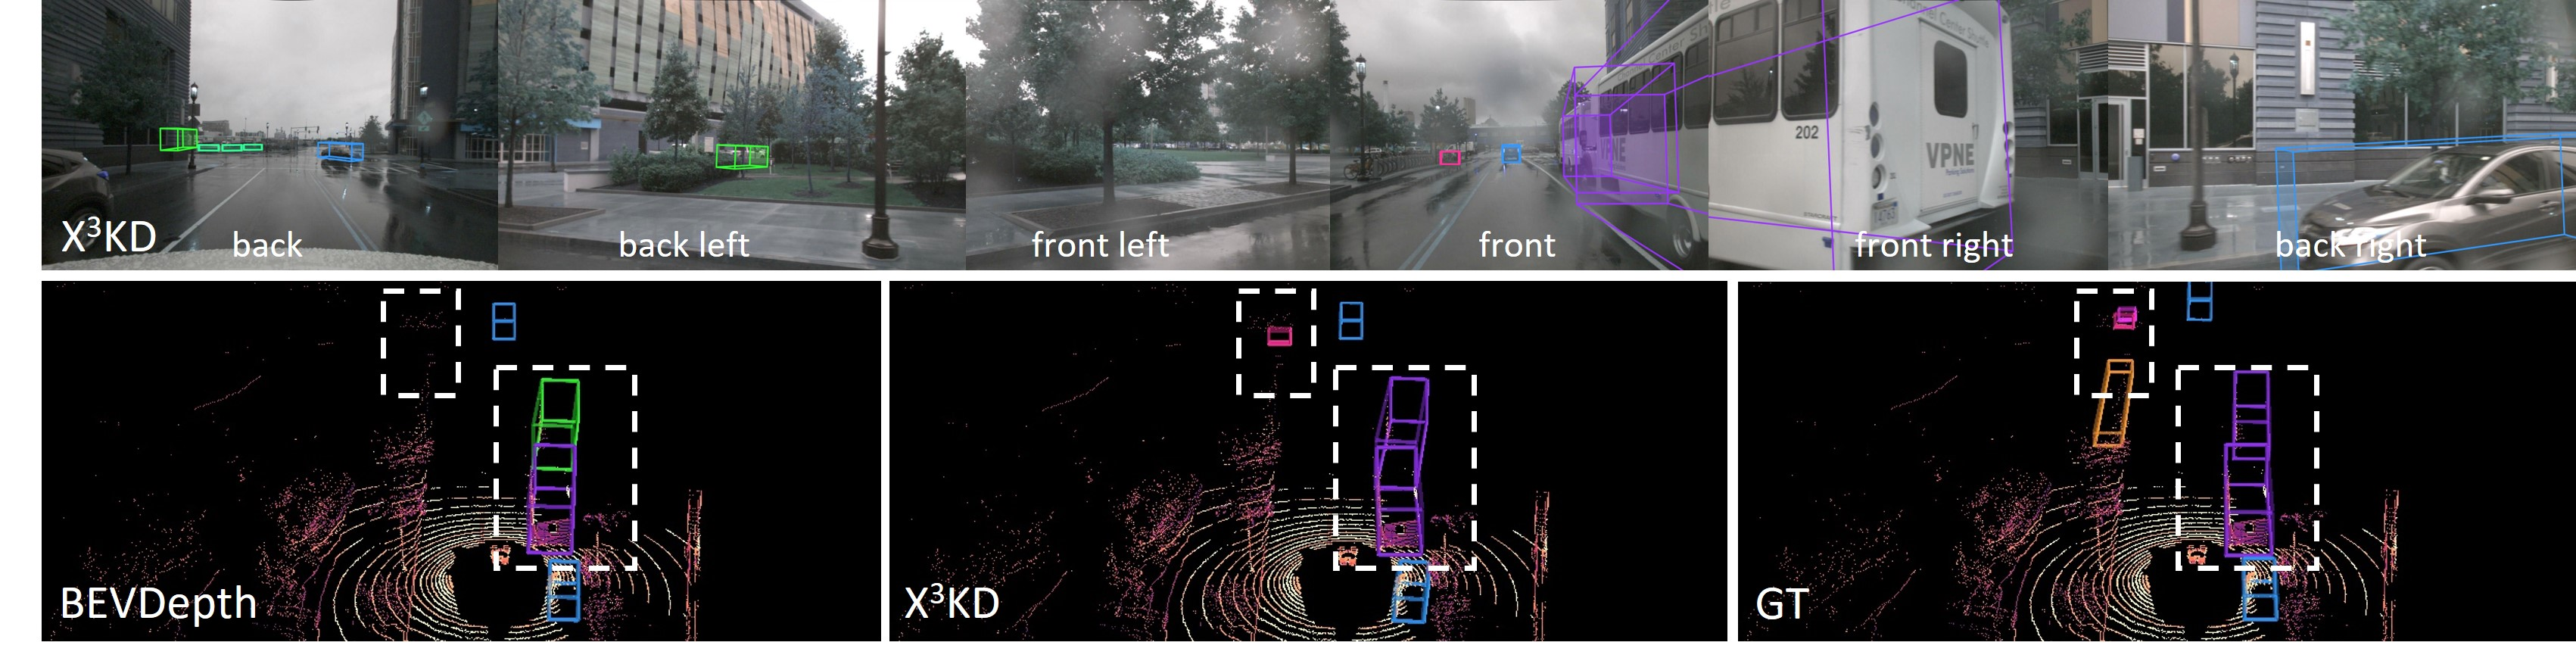}
    \includegraphics[width=0.96\linewidth]{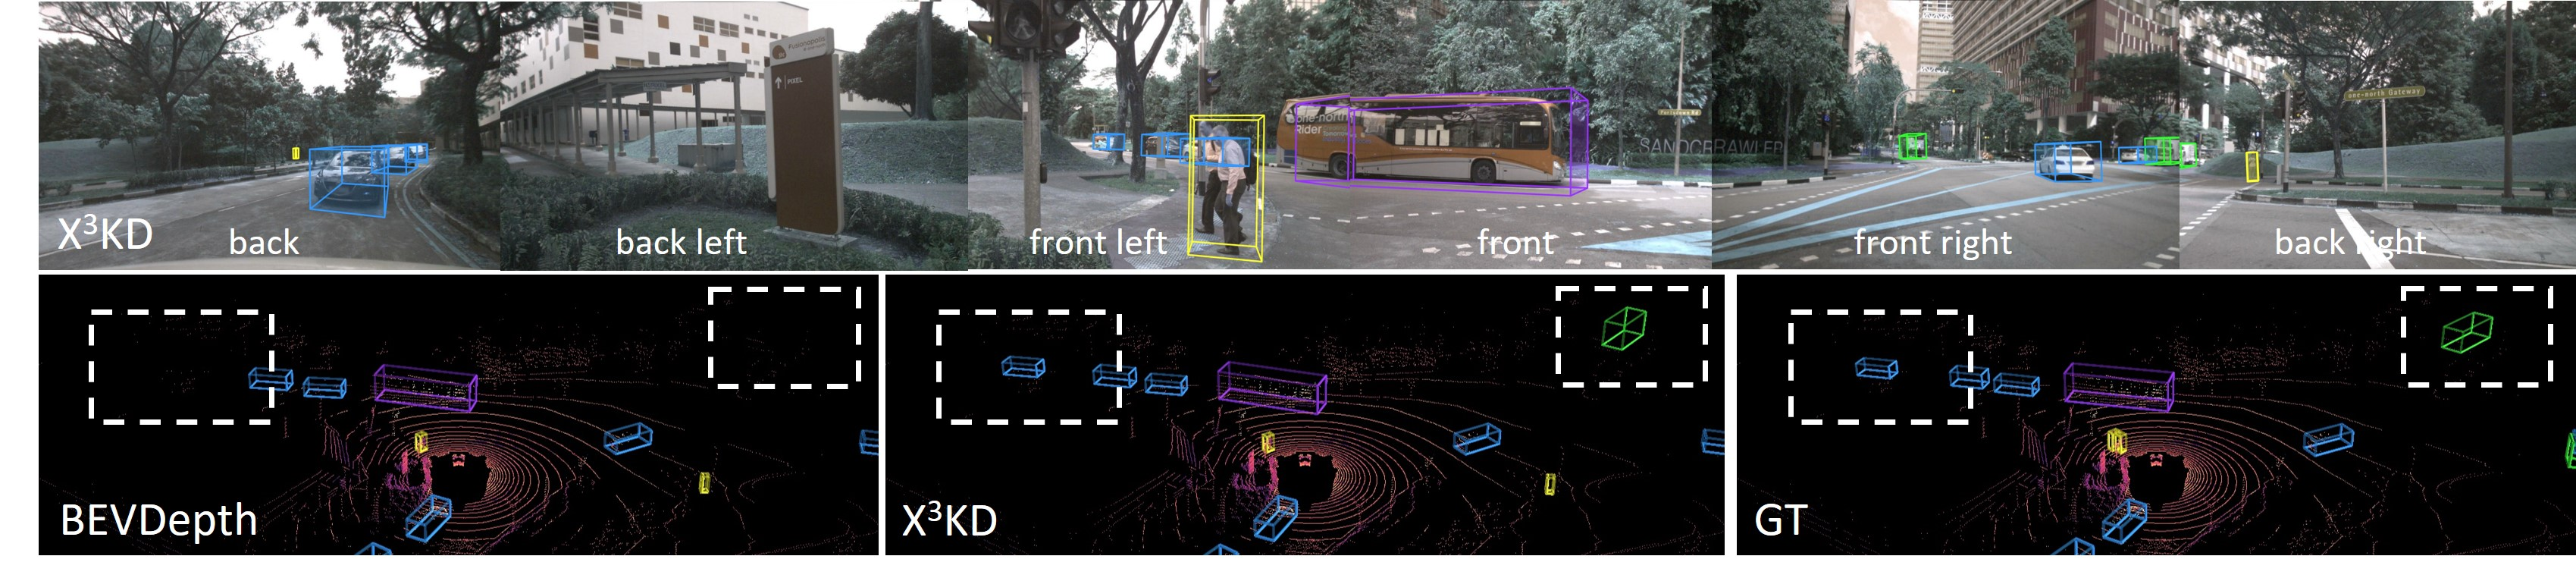}
    \includegraphics[width=0.96\linewidth]{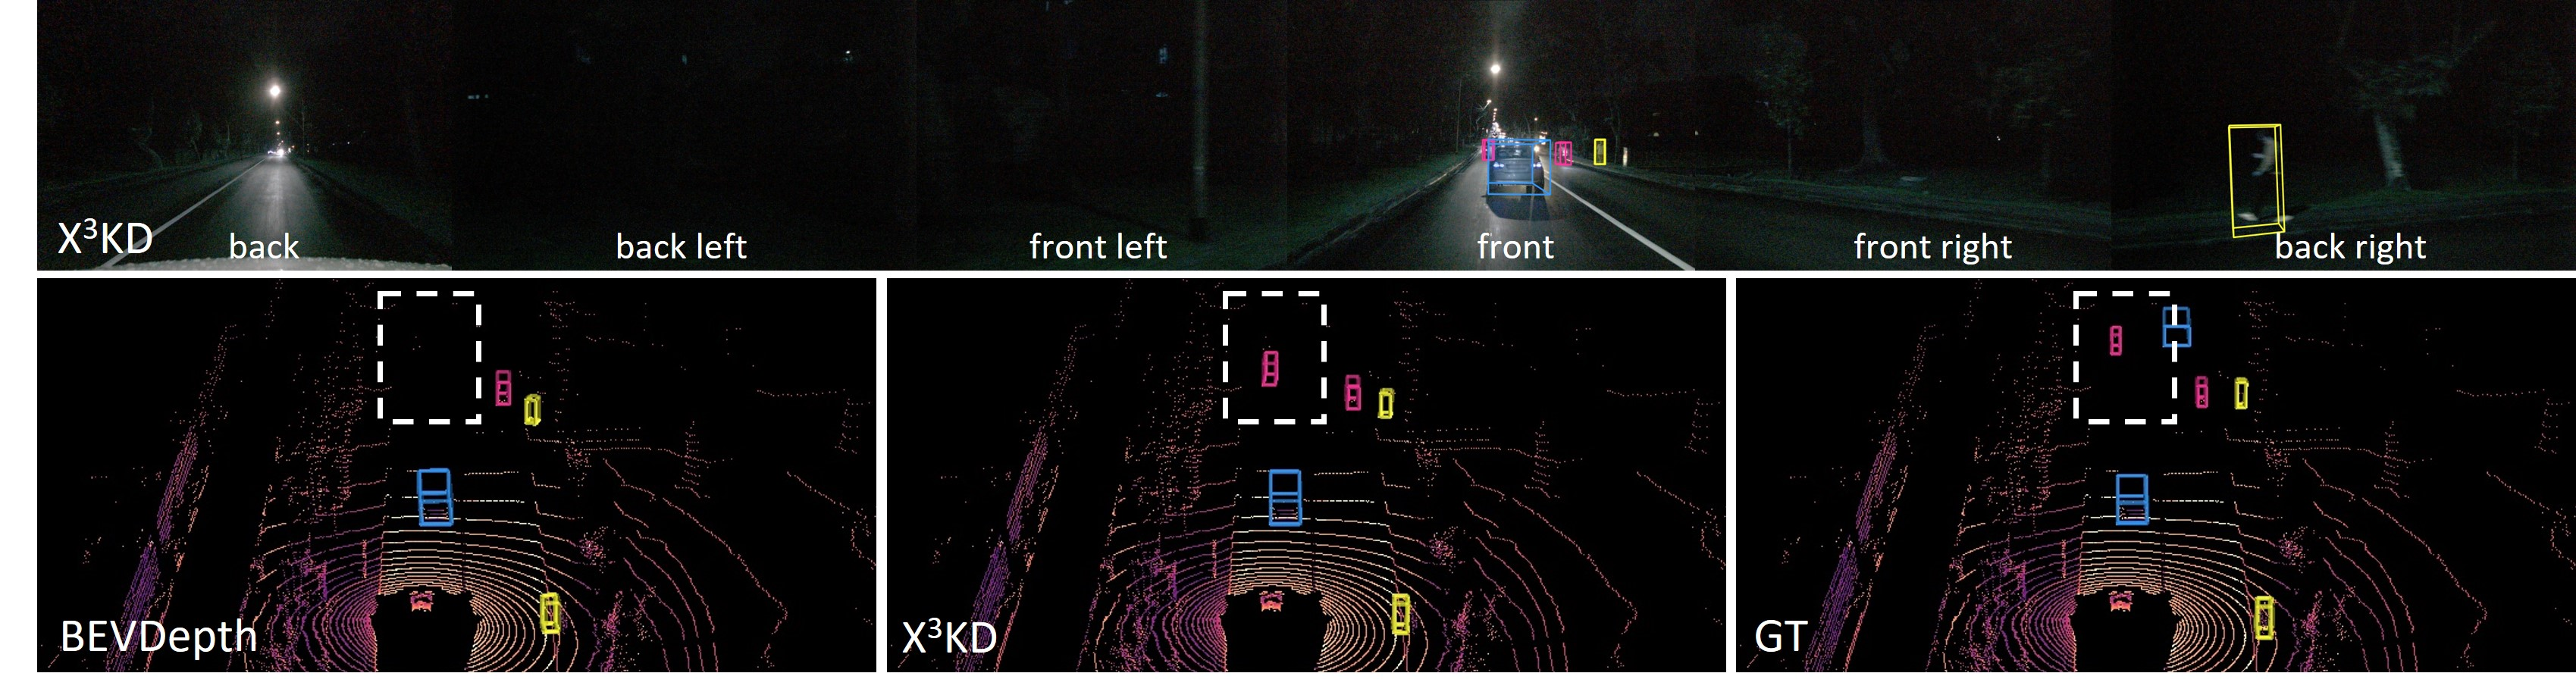}
    \includegraphics[width=0.96\linewidth]{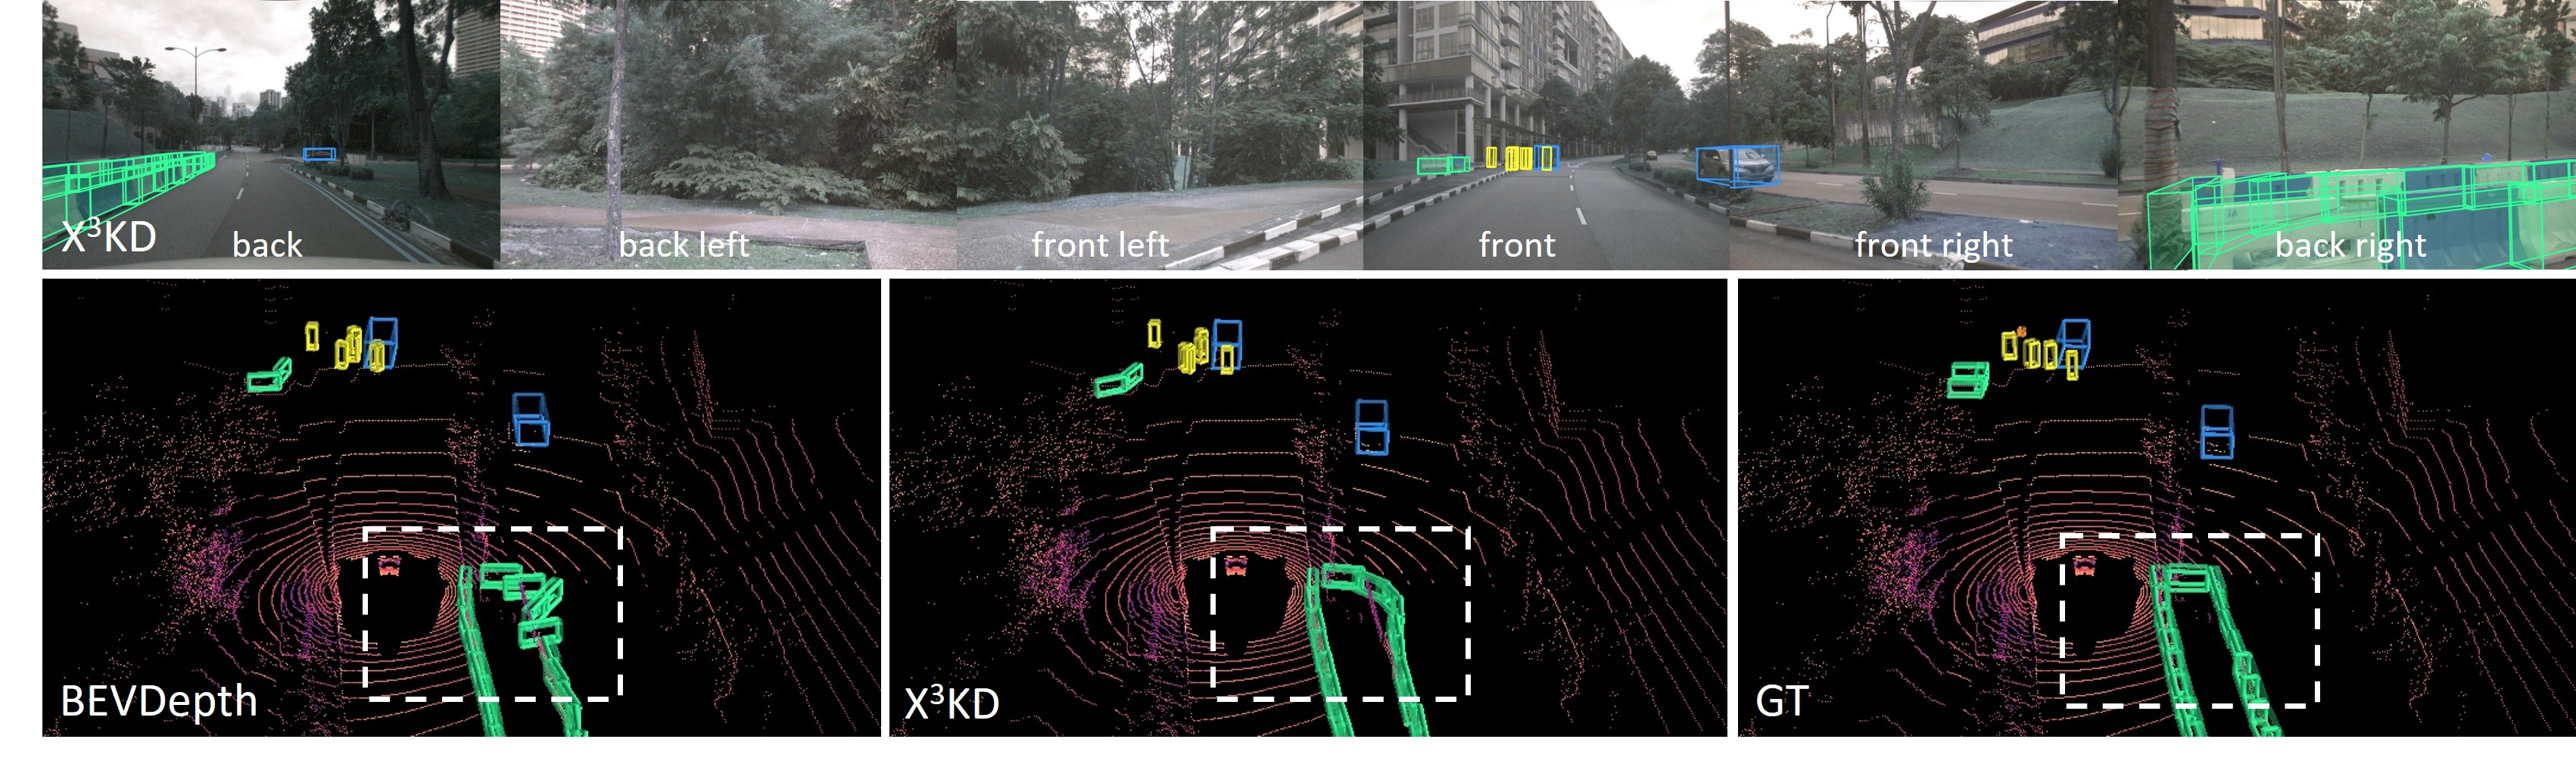}
    \vspace{-10pt}
    \caption{\textbf{Qualitative results on nuScenes}: We show the multi-camera input (top) and bounding box visualizations (bottom). We compare ResNet-101-based X$^3$KD$_\text{all}$ to BEVDepth$^\dagger$ and the ground truth (GT) for a resolution of $640 \times 1600$. Best viewed on screen and in color.}
    \label{fig:qualitative-supp}
\end{figure*}

We provide additional qualitative examples for X$^3$KD in comparison to the baseline BEVDepth$^\dagger$ and the ground truth (GT) in Fig.~\ref{fig:qualitative-supp}. In the first example from the top, we observe that the orientation of trucks and trailers (red and green boxes) is not well predicted by the baseline BEVDepth$^\dagger$ and some objects are not detected at all. While the predictions of X$^3$KD are also not perfect, most objects are detected and the orientation of objects is better aligned, which is also apparent by comparing the X$^3$KD output to the GT. We attribute the better detection to the additional guidance from instance segmentation in PV, while a better orientation and prediction in bird's eye view (BEV) is likely due to guidance from the LiDAR-based 3DOD model. More examples of objects that are difficult to  detect are given in the second and third example. In the second example, the bicycle (pink box) is quite far away and appears rather small in the front camera image. Similarly, in the third example the truck (green box) and the car (blue box) appear small and the car is partially occluded. Guidance from instance segmentation in perspective view can help to detect these rather difficult examples. This improved detection behavior also generalizes to adverse weather conditions as can be seen in the fourth example. Again, a bicycle is detected by X$^3$KD but not by the baseline BEVDepth$^\dagger$. Finally, the fifth example provides additional evidence on how the guidance from the LiDAR-based 3DOD teacher improves the translation and orientation characteristics of the predicted bounding boxes. The barriers (light green boxes) in BEVDepth$^\dagger$ are oriented rather random, while there is a structurally meaningful orientation observable for X$^3$KD.
