# Supplementary material for: X$^3$KD: Knowledge Distillation Across Modalities, Tasks and Stages for Multi-Camera 3D Object Detection
Source: arXiv:2303.02203 source file (2023-03-03)
Supplement: Supplementary file 3 [file supp_backbones.tex]

\begin{table}[t]
    \captionsetup{font=small, belowskip=-11pt}
    \footnotesize
    \centering
    \setlength{\tabcolsep}{7.0pt}
    \begin{tabular}{l|cc|cc}
        \toprule
        \textit{Model} 
        &  \textit{Backbone} 
        & \textit{Resolution}
        & \cellcolor[HTML]{ab9ac0}\textit{mAP}$\uparrow$ 
        & \cellcolor[HTML]{a5eb8d}\textit{NDS}$\uparrow$ \\
        \midrule
        BEVDepth$^\dagger$ & ResNet-50 & $256\times 704$ & 35.9 & 47.2 \\
        \rowcolor{gray8} \textbf{X$^3$KD} (Ours) & ResNet-50 & $256\times 704$ & \textbf{39.0} & \textbf{50.5} \\
        \midrule
        BEVDepth$^\dagger$ & ConvNeXt-T & $256\times 704$ & 38.3 & 50.8 \\
        \rowcolor{gray8} \textbf{X$^3$KD} (Ours) & ConvNeXt-T & $256\times 704$ & \textbf{39.7} & \textbf{51.9} \\
        \midrule
        BEVDepth$^\dagger$ & ResNet-101 & $640\times 1600$ & 42.8 & 53.6 \\
        \rowcolor{gray8} \textbf{X$^3$KD} (Ours) & ResNet-101 & $640\times 1600$ & \textbf{46.1} & \textbf{56.7} \\
        \bottomrule
    \end{tabular}\vspace{-5pt}
    \caption{\textbf{Ablation on varying backbones}: We show that X$^3$KD improves ResNet-based as well as ConvNeXt-based models on top of BEVDepth$^\dagger$ (re-implementation of~\cite{li2022bevdepth}).}
    \label{tab:supp-ablation-backbones}
\end{table}
