# Supplementary material for: X$^3$KD: Knowledge Distillation Across Modalities, Tasks and Stages for Multi-Camera 3D Object Detection
Source: arXiv:2303.02203 source file (2023-03-03)
Supplement: Supplementary file 4 [file supp_hyperparameters.tex]

\begin{table}[t]
    \captionsetup{font=small, belowskip=-6pt}
    \footnotesize
    \centering
    \setlength{\tabcolsep}{12.3pt}
    \begin{tabular}{l|cc|cc}
        \toprule
        \textit{Model} 
        &  Pre. 
        & $\lambda^{\text{X-AT}}$
        & \cellcolor[HTML]{ab9ac0}\textit{mAP}$\uparrow$ 
        & \cellcolor[HTML]{a5eb8d}\textit{NDS}$\uparrow$ \\
        \midrule
        BEVDepth$^\dagger$ & \ch & $0$ & 37.7 & 49.5 \\
        & \ch & $1$ & 37.6 & 49.4 \\
        \rowcolor{gray85} X-AT & \ch & $10$ & \textbf{37.9} & \textbf{49.8} \\
        & \ch & $20$ & 37.8 & 49.7 \\
        \bottomrule
    \end{tabular}\vspace{-5pt}
    \caption{\textbf{Ablation on the X-AT loss weight}. We initialize all models with backbones pre-trained on nuImages (Pre.).}
    \label{tab:supp-ablation-x-at}
\end{table}

\begin{table}[t]
    \captionsetup{font=small, belowskip=-6pt}
    \footnotesize
    \centering
    \setlength{\tabcolsep}{12.3pt}
    \begin{tabular}{l|cc|cc}
        \toprule
        \textit{Model} 
        &  Pre. 
        & $\lambda^{\text{X-FD}}$
        & \cellcolor[HTML]{ab9ac0}\textit{mAP}$\uparrow$ 
        & \cellcolor[HTML]{a5eb8d}\textit{NDS}$\uparrow$ \\
        \midrule
        BEVDepth$^\dagger$ & \ch & $0$ & 37.7 & 49.5 \\
        & \ch & $2$ & 37.8 & 49.6 \\
        \rowcolor{gray85} X-FD & \ch & $10$ & \textbf{38.2} & \textbf{50.0} \\
        & \ch & $25$ & 38.1 & 49.7 \\
        & \ch & $100$ & 37.3 & 48.8 \\
        \bottomrule
    \end{tabular}\vspace{-5pt}
    \caption{\textbf{Ablation on the X-FD loss weight}. We initialize all models with backbones pre-trained on nuImages (Pre.).}
    \label{tab:supp-ablation-x-fd}
\end{table}
