# Supplementary material for: X$^3$KD: Knowledge Distillation Across Modalities, Tasks and Stages for Multi-Camera 3D Object Detection
Source: arXiv:2303.02203 source file (2023-03-03)
Supplement: Supplementary file 5 [file supp_hyperparameters2.tex]

\begin{table}[t]
    \captionsetup{font=small, belowskip=-6pt}
    \footnotesize
    \centering
    \setlength{\tabcolsep}{11.3pt}
    \begin{tabular}{l|cc|cc}
        \toprule
        \textit{Model} 
        &  Pre. 
        & $\alpha^{\text{3D-bbox}}$
        & \cellcolor[HTML]{ab9ac0}\textit{mAP}$\uparrow$ 
        & \cellcolor[HTML]{a5eb8d}\textit{NDS}$\uparrow$ \\
        \midrule
        BEVDepth$^\dagger$ & \ch & \nap & 37.7 & 49.5 \\
        & \ch & $0.8$ & 37.9 & 49.8 \\
        \rowcolor{gray85} X-OD & \ch & $0.6$ & \textbf{38.1} & \textbf{50.0} \\
        & \ch & $0.3$ & 38.0 & 49.9 \\
        \bottomrule
    \end{tabular}\vspace{-5pt}
    \caption{\textbf{Ablation on the X-OD ground truth selection threshold}. We initialize all models with backbones pre-trained on nuImages (Pre.).}
    \label{tab:supp-ablation-x-od}
\end{table}

\begin{table}[t]
    \captionsetup{font=small, belowskip=-6pt}
    \footnotesize
    \centering
    \setlength{\tabcolsep}{11.3pt}
    \begin{tabular}{l|cc|cc}
        \toprule
        \textit{Model} 
        &  Pre. 
        & $\alpha^{\text{2D-bbox}}$
        & \cellcolor[HTML]{ab9ac0}\textit{mAP}$\uparrow$ 
        & \cellcolor[HTML]{a5eb8d}\textit{NDS}$\uparrow$ \\
        \midrule
        BEVDepth$^\dagger$ & \ch & $1.0$ & 37.7 & 49.5 \\
        & \ch & $0.8$ & 37.9 & 49.8 \\
        & \ch & $0.5$ & 38.0 & 50.0 \\
        \rowcolor{gray85} X-IS & \ch & $0.2$ & \textbf{38.7} & \textbf{50.1} \\
        & \ch & $0.1$ & 38.2 & 49.9 \\
        \bottomrule
    \end{tabular}\vspace{-5pt}
    \caption{\textbf{Ablation on the X-IS ground truth selection threshold}. We initialize all models with backbones pre-trained on nuImages (Pre.).}
    \label{tab:supp-ablation-x-is}
\end{table}
