# Supplementary material for: X$^3$KD: Knowledge Distillation Across Modalities, Tasks and Stages for Multi-Camera 3D Object Detection
Source: arXiv:2303.02203 source file (2023-03-03)
Supplement: Supplementary file 6 [file supp_more_baselines.tex]

\begin{table}[t]
    \captionsetup{font=small, belowskip=-8pt}
    \centering
    \footnotesize
    \setlength{\tabcolsep}{2.1pt}
    \setlength{\aboverulesep}{-0.3pt}
    \setlength{\belowrulesep}{1.0pt}
    \begin{tabular}{l|c|c|c|c}
        \toprule
        model & BEVDet & BEVDet + X$^3$KD & BEVDet4D & BEVDet4D + X$^3$KD \\
        \midrule
        \cellcolor[HTML]{a5eb8d}\textit{NDS}$\uparrow$ & 37.9 & 41.3 & 45.7 & 49.1 \\
        \bottomrule
    \end{tabular}
    \vspace{-8pt}
    \caption{Combination of X$^3$KD with BEVDet and BEVDet4D.}
    \label{tab:transferability}
\end{table}
