# Supplementary material for: X$^3$KD: Knowledge Distillation Across Modalities, Tasks and Stages for Multi-Camera 3D Object Detection
Source: arXiv:2303.02203 source file (2023-03-03)
Supplement: Supplementary file 7 [file supp_train_comp.tex]

\begin{table}[t]
    \captionsetup{font=small, belowskip=-15pt}
    \centering
    \footnotesize
    \setlength{\tabcolsep}{2.4pt}
    \setlength{\aboverulesep}{-0.3pt}
    \setlength{\belowrulesep}{1.0pt}
    \begin{tabular}{l|c|cccc|c}
        \toprule
        model & BEVDepth & X-AT & X-FD & X-OD & X-IS & \textbf{X$^3$KD} \\
        \midrule
        training time & \SI{54}{h} & \SI{65}{h} & \SI{65}{h} & \SI{67}{h} & \SI{73}{h} & \SI{78}{h} \\
        GPU memory & \SI{39}{GB} & \SI{44}{GB} & \SI{44}{GB} & \SI{44}{GB} & \SI{48}{GB} & \SI{52}{GB} \\
        \midrule
        \cellcolor[HTML]{a5eb8d}\textit{NDS}$\uparrow$ & 47.2 & 48.1 & 48.5 & 48.7 & 50.1 & 50.5 \\
        \bottomrule
    \end{tabular}
    \vspace{-8pt}
    \caption{Training complexity/performance trade-off when training on 4 NVIDIA A100 GPUs with a batch size of 16 per GPU.}
    \label{tab:train-complexity}
\end{table}
